# Supplementary material for: Normalizing Flow-based Neural Process for Few-Shot Knowledge Graph Completion
Source: arXiv:2304.08183 source file (2023-04-17)
Supplement: Supplementary file 1 [file appendix.tex]

\section{Appendix}

\subsection{Importance of FKGC in Web}\label{sec:web}
Knowledge Graphs (KGs), as a form of structured knowledge representation, have been widely applied in Web applications \cite{xiong2017explicit,wang2019knowledge,cao2019efficient}. Meanwhile, with the development of the Web, KGs have also been considered as a fundamental infrastructure in Web3.0 \cite{chen2021openkg,yan2019differentiated}. However, in real-world, KGs are usually incomplete, which requires practitioners to complete missing facts by inferring from existing ones. What is more, a large portion of relations in KGs follow a long-tail distribution with less than 10 associated facts \cite{xiong2018one}, which largely limits the applications of existing methods \cite{nickel2011three,bordes2013translating}. Thus, few-shot knowledge graph completion (FKGC) studied in this paper, aiming to predict missing facts with few-shot associated facts \cite{xiong2018one,zhang2020few}, essentially addresses a core challenge of the Web -- \textbf{improving core web technologies} with knowledge graph completion, to enable the \textbf{Web as a technical infrastructure} for Web applications.

\subsection{Attentive Relation Message Passing}\label{sec:arpgnn}
In this section, we illustrate the details of attentive relation message passing. As shown in Fig.~\ref{fig:message}, (1) we first synthesize the representation of each neighbor relation and (2) aggregate the relation representation attentively. Intuitively, the GNN message passing is essentially a simulation of BFS, which exhibits the ability to capture paths between nodes. By using the GNN, we can excavate the parallel computation ability of GPUs to accelerate the process of path extraction. Besides, the ARP-GNN can also differentiate the contribution of each relation in the path by using the attention mechanism.

\begin{figure}[htbp]
    \centering
    \includegraphics[width=0.4\columnwidth,trim=0 0 0cm 0, clip]{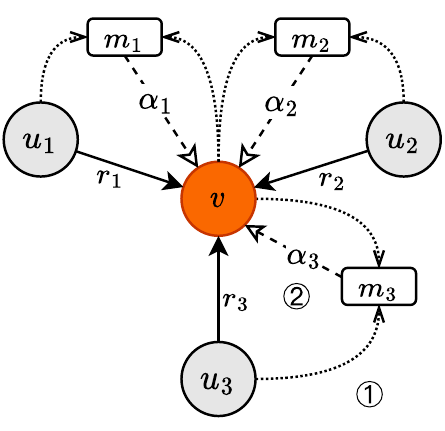}
    \caption{The illustration of attentive relation message passing. }
    \label{fig:message}
\end{figure}

\subsection{Training Algorithm of \ourmethod.}\label{sec:training}
We illustrate the training process is shown in Algorithm \ref{alg:FKGC}. In training, we first generate the relation representation $r'$ using ARP-GNN. Then, we generate the prior distribution $P(z|\mathcal{C}_r)$ from the context data using neural process encoder. Since we want the generated distribution to incorporate both the context data and target data. We apply the normalizing flow and neural process encoder to both the context data $\mathcal{C}_r$ and target data $\mathcal{D}_r$ to estimate the posterior distribution. Finally, we optimize the parameters of \ourmethod using the ELBO loss.

%-----------------------------
\begin{algorithm}[htbp]
    \caption{The training process of \ourmethod}\label{alg:FKGC}
    \KwIn {Training relations $\mathcal{R}_{train}$; knowledge graph $\mathcal{G}$.}
    \KwOut {Model parameters $\Theta$}
    \While{not done}{
        Sample a relation $\mathcal{T}_r=\{\mathcal{C}_r,\mathcal{D}_r\}$ from $\mathcal{R}_{train}$\;
        Generate relation representation $r'$ (Eq. 5-13)\;
        Generate prior distribution $P(z|\mathcal{C}_r)$ using $\mathcal{C}_r$ (Eq. 14-18)\;
        Generate target base distribution $Q_0(z_0|\mathcal{C}_r,\mathcal{D}_r)$ using $\mathcal{C}_r$ and $\mathcal{D}_r$ (Eq. 14-18)\;
        Sample a $z_0$ from the base distribution $Q_0(z_0|\mathcal{C}_r,\mathcal{D}_r)$ \;
        Apply NF to generate $z_T$ (Eq. 19)\;
        Optimize $\Theta$ using the ELBO loss (Eq. \ref{eq:loss})\; 
    }
\end{algorithm}
%-----------------------------

\subsection{Datasets}\label{app:dataset}
In experiments, we use three benchmark datasets: NELL, WIKI, and FB15K-237, and split the datasets following the public settings. The NELL and WIKI dataset can be accessed from this link\footnotemark[4], and FB15K-237 can be downloaded from this link\footnote{\url{https://github.com/SongW-SW/REFORM}}. The split of the one-to-one and one-to-many relations can be obtained from this link\footnotemark[8]. The statistics of the one-to-one and one-to-many relations in the NELL dataset are shown in Table \ref{tab:n-1} and Table \ref{tab:n-n}, respectively. For relations like \textit{co\_author}, they have many head entities to many tail entities (i.e., \textit{many-to-many}). We can decompose them into multiple one-to-one or one-to-many FKGC tasks by fixing the head entity and predicting the tails. Thus, we do not list many-to-many relations in experiments.

\begin{table*}
    \centering
    \caption{Statistics of the one-to-one relations in the NELL dataset.}
    \label{tab:n-1}
    %\resizebox{\linewidth}{!}{%
    \begin{tabular}{ccc} 
    \toprule
    Relation                               & \#Query & Example                                                    \\\midrule
    sportsgamesport                        & 74      & (n1937\_world\_series, sportsgamesport, baseball)            \\
    geopoliticallocationresidenceofpersion & 143     & (barack\_obama, geopoliticallocationresidenceofpersion, us)  \\
    producedby                             & 213     & (civic\_hybrid, producedby, honda)                          \\
    \bottomrule
    \end{tabular}
    %}
\end{table*}

\begin{table*}
    \centering
    \caption{Statistics of the one-to-many relations in the NELL dataset.}
    \label{tab:n-n}
    %\resizebox{\linewidth}{!}{%
    \begin{tabular}{ccc} 
    \toprule
    Relation                           & \#Query & Example                                                       \\\midrule
    automobilemakerdealersincity       & 178     & (lexus, automobilemakerdealersincity, dallas/columbus/austin...)                   \\
    athleteinjuredhisbodypart          & 69      & (peter\_moylan, athleteinjuredhisbodypart, shoulders/fingers/hands)           \\
    politicianusendorsespoliticianus   & 386     & (chris\_dodd, politicianusendorsespoliticianus, barack\_obama/clinton)  \\
    animalsuchasinvertebrate           & 415     & (insects, animalsuchasinvertebrate, bugs/flies/snails...)                  \\
    sportschoolincountry               & 103     & (america, sportschoolincountry, soccer/skiing/hockey...)                         \\
    agriculturalproductcamefromcountry & 140     & (india, agriculturalproductcamefromcountry, sweets/wood/wool...)             \\
    automobilemakerdealersincountry    & 96      & (uk, automobilemakerdealersincountry, lotus/lexus/gmc...)                    \\
    \bottomrule
    \end{tabular}
    %}
    \end{table*}

\subsection{Baselines}\label{sec:baselines}
We select four models (e.g., TransE \cite{bordes2013translating}, TransH \cite{wang2014knowledge}, DistMult \cite{bordes2014semantic}, and ComplEx \cite{trouillon2016complex}) as the traditional KGC baselines. These baselines can be implemented using the open-source code\footnote{\url{https://github.com/thunlp/OpenKE/tree/OpenKE-Tensorflow1.0}}.
\begin{itemize}
    \item TransE \cite{bordes2013translating} represents entities and relations in a $d$-dimension vector space following the translational principle. 
    \item TransH \cite{wang2014knowledge} models a relation as a hyperplane, which enables to handle complex relations.
    \item DistMult \cite{bordes2014semantic} proposes a bilinear formulation to calculate the semantic similarity.
    \item ComplEx \cite{trouillon2016complex} adopts the complex-valued embeddings to handle the symmetric and antisymmetric relations.
\end{itemize}

We select five FKGC methods, including GMatching\footnote{\url{https://github.com/xwhan/One-shot-Relational-Learning}} \cite{xiong2018one}, MetaR\footnote{\url{https://github.com/AnselCmy/MetaR}} \cite{chen2019meta}, FSRL\footnote{\url{https://github.com/chuxuzhang/AAAI2020_FSRL}} \cite{zhang2020few}, FAAN\footnote{\url{https://github.com/JiaweiSheng/FAAN}} \cite{sheng2020adaptive}, and GANA\footnote{\url{https://github.com/ngl567/GANA-FewShotKGC}} \cite{niu2021relational}.
\begin{itemize}
    \item GMatching \cite{xiong2018one} proposes a neighbor encoder and a LSTM matching network to calculate the similarity.
    \item MetaR \cite{chen2019meta} is a meta-learning-based method that uses a meta-learner to capture the relation-specific representation.
    \item FSRL \cite{zhang2020few} proposes a LSTM encoder to summarize the support set information.
    \item FAAN \cite{sheng2020adaptive} proposes a relation-specific attention aggregator and a transformer-based support set encoder to generate the relation representation.
    \item GANA \cite{niu2021relational} integrate the meta-learning and TransH to consider the complex relations, which is considered as the state-of-the-art FKGC baseline.
\end{itemize}

The implementation of these methods can be obtained from the repositories publicized by authors. In NELL and FB15K-237, these methods follow the same settings, we directly use results reported by these papers to avoid re-implementation bias. In FB15K-237, we use the code publicized by authors to conduct experiments.

\subsection{Implementation Details}\label{sec:implementation}
The batch size is set to 128 for NELL and FB15K-237, but 64 for WIKI due to the limitation of GPU memory. We use the Adam optimizer and early stopping on MRR with 3 patience steps to avoid over-fitting. We develop our model using the PyTorch\footnote{\url{https://pytorch.org/}} and DGL\footnote{\url{https://www.dgl.ai/}}. For NELL and FB15K-237 datasets, the experiments are conducted on RTX3090 GPU with 32GB system memory. For WIKI dataset, the experiments are conducted on a single NVIDIA Tesla A100 GPU with 128GB system memory. The code of \ourmethod is available at this link\footnote{\url{https://anonymous.4open.science/r/NP-FKGC-80E0/}}.
